# Supplementary material for: Stochastic Methods in Variational Inequalities: Ergodicity, Bias and Refinements
Source: arXiv:2306.16502 source file (2023-06-28)
Supplement: Supplementary file 3 [file Appendix-CLT.tex]

% !TEX root = ../Arxiv-Main.tex

\begin{theorem}\label{thm:CLT}
    Let the \cref{asm:solutionset,asm:lipschitz-lineargrowth,asm:wqsm,asm:oracle,asm:uniformbound} hold. Then for a test function $\tf$ and the choice of step-sizes specified in \cref{thm:close} we have that 
    \begin{equation}
    \nRuns^{-1/2}S_\nRuns(\tf) \to \normal(0,\sdev^2_\pi(\tf))
    \end{equation}
    where $S_\nRuns(\tf):= \sum_{\run=\start}^\nRuns \bracks{\tf(\state_\run)-\pi(\state)}$, $\pi(\tf):= \int\tf(\point)\dd \pi(\point)$ and $\sdev^2_\pi(\tf):= \lim_{\nRuns\to\infty}\frac{1}{\nRuns}\ex\bracks{S_{\nRuns}(\tf)}$
\end{theorem}
