# Supplementary material for: Stochastic Methods in Variational Inequalities: Ergodicity, Bias and Refinements
Source: arXiv:2306.16502 source file (2023-06-28)
Supplement: Supplementary file 4 [file notes.tex]

See also theorem 11.0.1
